# Supplementary material for: SCP: Soft Conditional Prompt Learning for Aerial Video Action Recognition
Source: arXiv:2305.12437 source file (2024-08-28)
Supplement: Supplementary file 1 [file 7-supplementary.tex]

\section{More Ablation Studies}
We conduct ablation studies on the effectiveness of experts number for learnable prompt, different inputs for the large vision model, and the effect of each component of our method on Okutama.
\subsection{Experts Number for Learnable Prompt}
In our proposed learnable prompt, it learns to dynamically generate prompts from a pool of prompt experts under different inputs. Prompt experts are learnable parameters that can be updated from the training process and they are input-invariant (prompt experts) prompts. which contain task information. In this section, we explore the effect of the number of experts. As shown in Table~\ref{tab:expert_num}, we evaluated various experts number including 4, 8, 16, and 32. From our experiment, PLAR with the expert number of 8 achieved the best accuracy.
\begin{table}[h]
\centering
\begin{tabular}{c c c }
\toprule
Method & Frame size  & Accuracy    \\
\midrule
Baseline & 224x224 & $71.54\%$  \\
Baseline + SCP with 4 Experts  & 224x224 & $76.16\%$  \\
Baseline + SCP with 8 Experts & 224x224 & $76.34\%$  \\
Baseline + SCP with 16 Experts & 224x224 & $75.93\%$  \\
Baseline + SCP with 32 Experts & 224x224 & $73.70\%$  \\
\bottomrule
\end{tabular}
\caption{Ablation study in terms of different experts number on the Okutama dataset. We evaluated various experts number including 4, 8, 16, and 32. From our experiment, with the expert number of 8 achieved better accuracy.}
\label{tab:expert_num}
\vspace{-4mm}
\end{table}

\subsection{Different Inputs for Large Vision Model}
In this work, we explore the possibility of using large vision models as the prompt to instruct the action recognition task. We use the output of SAM as our prompt. For the large vision model, we use Segment Anything Model (SAM~\citep{kirillov2023segment}), which can segment any object in an image given only some extra inputs like a single click or box. As shown in Tbale~\ref{tab:LVM_prompt}, for SAM's prompts, we tried single point, two points, four points (line), and bbox. From our experiment, the large vision model with bbox achieved better accuracy, which also means more detailed extra inputs will lead to better outputs,  further resulting in better prompts for our task.
\begin{table}[h]
\centering
\begin{tabular}{c c c }
\toprule
Method & Frame size  & Accuracy    \\
\midrule
Large Vision Model (SAM) with 1 point & 224x224 & $58.12\%$  \\
Large Vision Model (SAM) with 2 points & 224x224 & $58.02\%$  \\
Large Vision Model (SAM) with 4 points (Line) & 224x224 & $66.30\%$  \\
Large Vision Model (SAM) with bbox point & 224x224 & $74.68\%$  \\
\bottomrule
\end{tabular}
\caption{Ablation study in terms of different inputs for large vision model on the Okutama dataset. We evaluated various inputs including single point, two points, four points, and bbox. From our experiment, the large vision model with bbox achieved better accuracy.}
\label{tab:LVM_prompt}
\end{table}

\subsection{Effect of Each Component of Our Method}
We also evaluated the effect of the components in our methods, including ROI alignment (ROI), Large Vision Model, and Learnable Prompt. As shown in Table~\ref{tab:component}, ROI can achieve 2.07\% improvement, ROI combined with Large Vision Model can achieve 3.14\% improvement, ROI combined with our Learnable Prompt can achieve 4.80\% improvement. The experiments showed the effectiveness of our proposed methods.

\input{tables/component}
\subsection{Visualization}
For the large vision model, we visualize the outputs in terms of different prompts, including bbox, line, and points.  As shown in Figure~\ref{fig:mask}, bbox and line have more stable outputs, which means better prompts result in better outputs.

\begin{figure*}[t]
    \centering
    \includegraphics[width=\textwidth]{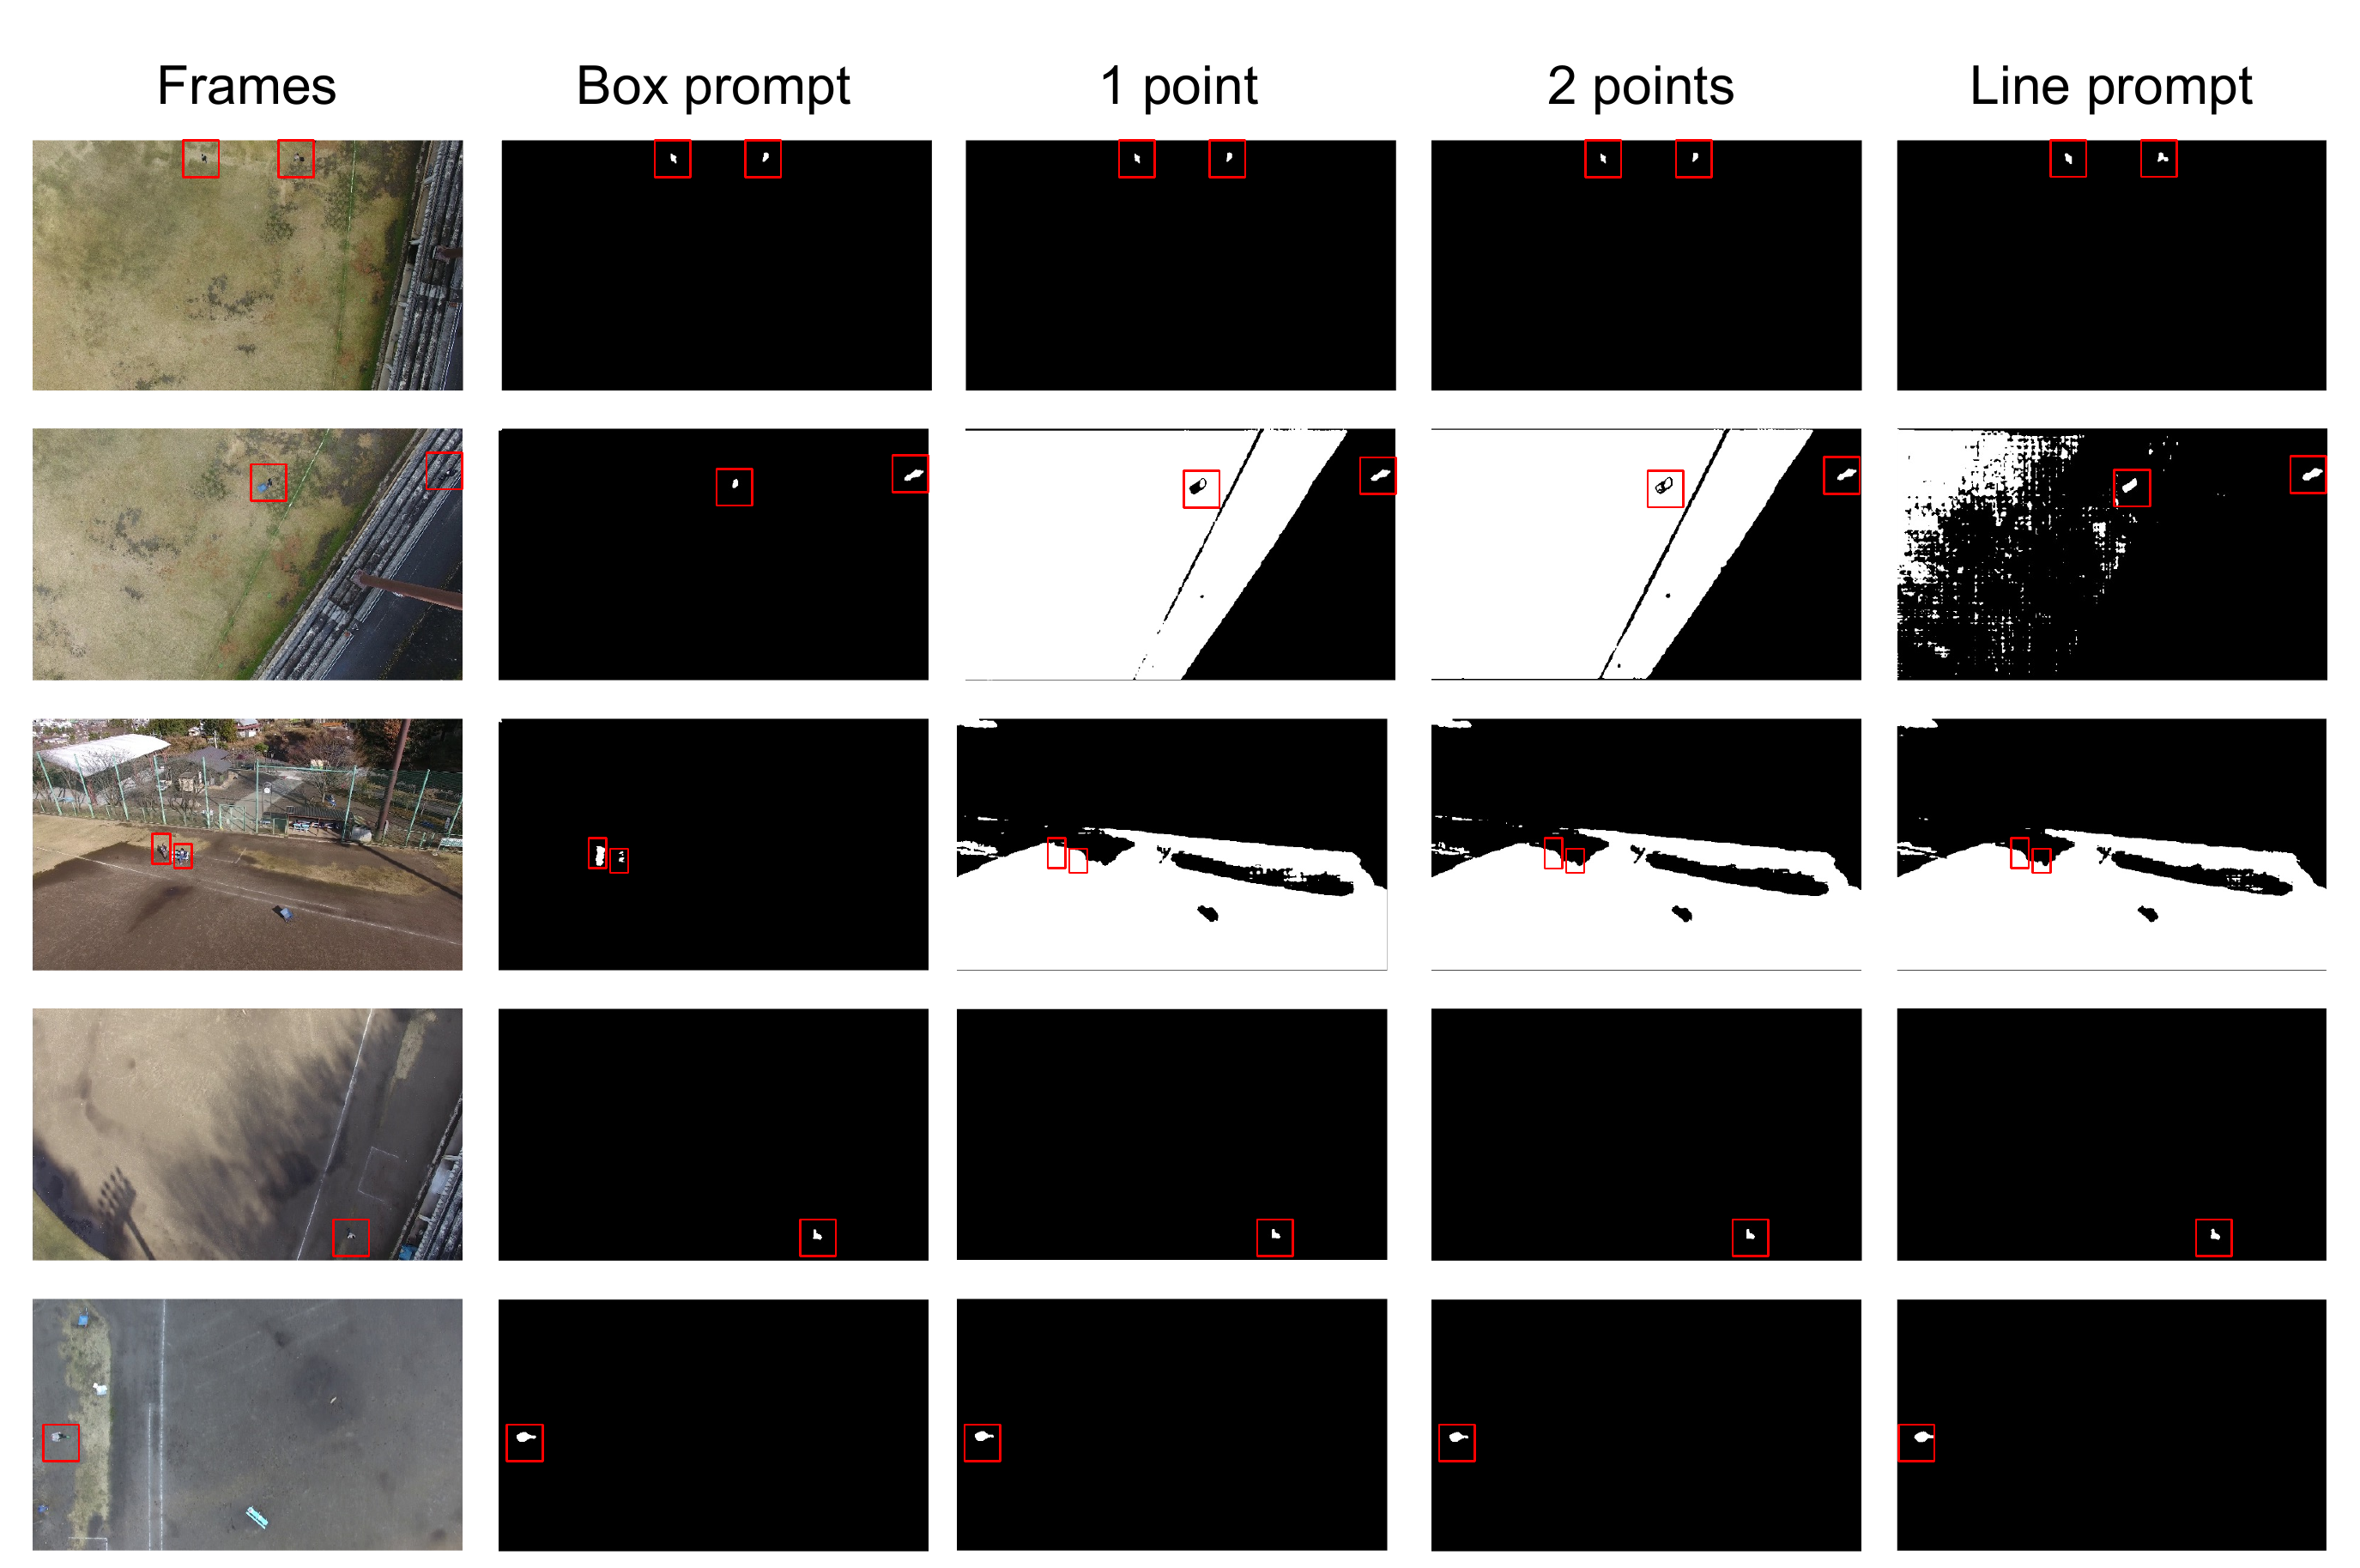}
    \caption{{\bf Large Vision Model:} Prompts from the large vision model, no supervision needed. We visualize the outputs in terms of different prompts, including bbox, line, and different points. bbox and line have more stable outputs, which means better prompts result in better outputs.}
    \label{fig:mask} 
    \vspace{-5mm}
\end{figure*}

\section{Experiment Settings}
All experiments are conducted on a desktop equipped with 8 Nvidia A5000 GPUs.

\textbf{Okutama:} For the multi-agent experiments, all the frames extracted from the video datasets were scaled to 224 × 224. The backbone is Swin-T~\citep{liu2021swin}. Following \citep{yadav2023droneattention}, the feature maps obtained were processed in the ROIAlign function (crop size of 5 × 5) to get the desired ROIs. Then we used the fully connected layer to encode those features to classifier features. The one-hot encoded targets and classifier features were fed into Binary Cross Entropy Logits Loss. Other training settings follow \citep{liu2021swin}.

\textbf{Something-something v2:} Following ~\citep{li2022mvitv2}, we fine-tune the pre-trained Kinetics models. Specifically, we train for 100 epochs using 8 GPUs with a batch size of 64 and a base learning rate of 5e-5 with a cosine learning rate schedule. We use Adamw and use a weight decay of 1e-4 and a drop path rate of 0.4. For other training and testing settings, we follow ~\citep{li2022mvitv2}. And the backbone is MViTv2-S~\citep{li2022mvitv2}.

\textbf{NEC-Drone:} The initial learning rate is set at 0.1 for training from scratch and 0.05 for initializing with Kinetics pretrained weights. Stochastic Gradient Descent (SGD) is used as the optimizer with 0.0005 weight decay and 0.9 momentum. We use cosine/poly annealing for learning rate decay. Unless further specified, the videos are decoded as a single clip and all the frames are randomly scaled and center cropped to the size 224 × 224 during training. During testing, we scale the shorter spatial side to 256 and take 3 crops of 224 × 224 to cover the longer spatial axis. We average the scores for all individual predictions.
